# Supplementary material for: Capacitively-coupled resonators for terahertz planar-Goubau-line filters
Source: arXiv:2206.01485 source file (2022-11-09)
Supplement: Supplementary file 1 [file 9_Supplementary.tex]

% For restarting Figure reference counter
\renewcommand{\thefigure}{S\arabic{figure}}

\setcounter{figure}{0}


\section*{Supplementary material}

\subsection{Electromagnetic simulations}

Electromagnetic simulations of the device were carried out using a finite element method software (Ansys HFSS) to model the propagation of the field across the microfluidic loaded with the sample (Fig.~\ref{fig:simulation_setup}.a). The sample's permittivity values were swept in both real (from 1 to 7) and imaginary (from 0 to 6) part, and the resulting effective refractive index were collected, establishing the relation between the sample's refractive index and the effective refractive index.

The simulated CPW was excited with a rectangular waveguide port with height and width equal to $\SI{128}{\um}$ and $\SI{200}{\um}$, for the case of $\epsilon_s = 1 - j0$.
The port size would be scaled to keep a constant electrical size for each simulated sample.
The boundary face which contains each rectangular port was set equal to H-plane (Fig.~\ref{fig:simulation_setup}.a) according to Ansys HFSS Help guide, ensuring that at the boundaries of the port the electric field can only be tangential, and avoiding exciting other undesired modes. We also used an H-plane to account for the symmetries in the CPW and reduce simulation time.

\begin{figure}[h]
\centering
\includegraphics[width=0.24\textwidth]{fig/simulation_setup.pdf}
\includegraphics[width=0.24\textwidth]{fig/simulation_setup_boundaries.pdf}
% \includegraphics[width=2.5in]{fig/Transform_func.jpg}
% where an .eps filename suffix will be assumed under latex, 
% and a .pdf suffix will be assumed for pdflatex; or what has been declared
% via \DeclareGraphicsExtensions.
\caption{\textbf{3D electromagnetic  simulation environment.} (a) Simulation environment of the CPW with sample on top showing the waveguide ports which excite the CPW. The CPW's vertical symmetry was exploited and only half of the CPW was simulated with a H-plane symmetry, reducing computation time. (b) Visualisation of H-symmetry plane, and the H-plane boundaries used for the same face where the ports are. For the rest of the simulation environment faces, radiation boundaries were used.}
\label{fig:simulation_setup}
\end{figure}

\subsection{Calibration}

For calibrating our measurements we used dedicated multi-line Thru-Reflect-Line standards \cite{Marks1991b}, included in the substrate of the measured CPW.
The lines used for calibrating have electrical lengths of $\lambda/4$, $3\lambda/4$, and $11\lambda/4$ at the centre of our frequency band, approximately 910~GHz.
As a reflect, we terminated the CPW by short-circuiting the signal and ground planes.

\subsection{Noise floor and output power}
The noise floor of the measurements gives an indication of the system's dynamic range.
The noise floor was measured for two different calibration planes: (1) rectangular waveguide calibration (Short-Open-Load-Through ), at the interface between the frequency extenders and contact probes, and (2) CPW calibration, at the calibration plane used for measuring.
The noise floor was measured from $S_{21}$ when ports 1 and 2 were isolated, after applying each calibration.
Fig.~\ref{fig:DR}.a shows the values of the noise floor across frequency for each calibration.
The frequency-averaged dynamic range of the CPW calibration is  $\SI{-49}{dB}$, whereas for the rectangular waveguide calibration is $\SI{-69}{dB}$.
The noise floor could be further improved by using time-averaging techniques. Fig.~\ref{fig:DR}.b shows the output power across frequency for the frequency extenders used to measure, having at least $\SI{-44}{dBm}$ and $\SI{-39}{dBm}$ of power for each extender.


\begin{figure}[h]
\centering
\includegraphics[height=0.25\textwidth]{fig/noiseFloor.pdf}
\includegraphics[height=0.25\textwidth]{fig/power_VDI_freqExtenders.jpg}
\caption{\textbf{Measurement equipment has a high dynamic range across the band}. (a) Noise floor for the frequency extenders waveguide calibration and the CPW calibration. The frequency averaged dynamic range is 46~dB for CPW calibration and 69~dB for the frequency extender calibration. (b)~Output power across the frequency band for the frequency extenders, as shown in their specifications.}
\label{fig:noiseFloor}
\end{figure}


\subsection{S-parameters}

Two-port S-parameter measurements ($\text{S}_{11}$, $\text{S}_{12}$,  $\text{S}_{21}$, and   $\text{S}_{22}$), were measured in magnitude and phase between $\SI{0.75}{THz}$ and $\SI{1.1}{THz}$. Fig.~\ref{fig:raw_sParams} shows the results of the five-measurement average of the S-parameters.
The reflection coefficients, $\text{S}_{11}$ and $\text{S}_{22}$, have typical values bellow $\SI{-5}{dB}$, which is reasonable for a reflection in the air-PDMS-sample interfaces.
The reflection is deteriorated at the higher frequencies of the measured band, arguably as a consequence of lower SNR and lower quality of the calibration.
The magnitude of $\abs{S_{11}}$ are typically higher than the ones in $\abs{S_{22}}$, which could be due to different proving conditions.
The magnitude values of $\abs{S_{12}}$ are very similar to the values of $\abs{S_{21}}$ (Fig.~\ref{fig:raw_sParams}.c-d), as expected from reciprocal passive structures.
Additionally, the magnitude values decreases for increased water concentration of the samples, since water is lossier than IPA.
The phases of ${S_{12}}$ and ${S_{21}}$ also show to follow a steady trend with the change of IPA concentration.

\begin{figure}[H!]
\centering
\includegraphics[width=0.24\textwidth]{fig/S11_mag.pdf}
\includegraphics[width=0.24\textwidth]{fig/S22_mag.pdf}\\
\includegraphics[width=0.24\textwidth]{fig/S12_mag.pdf}
\includegraphics[width=0.24\textwidth]{fig/S21_mag.pdf}\\
\includegraphics[width=0.24\textwidth]{fig/S12_phase.pdf}
\includegraphics[width=0.24\textwidth]{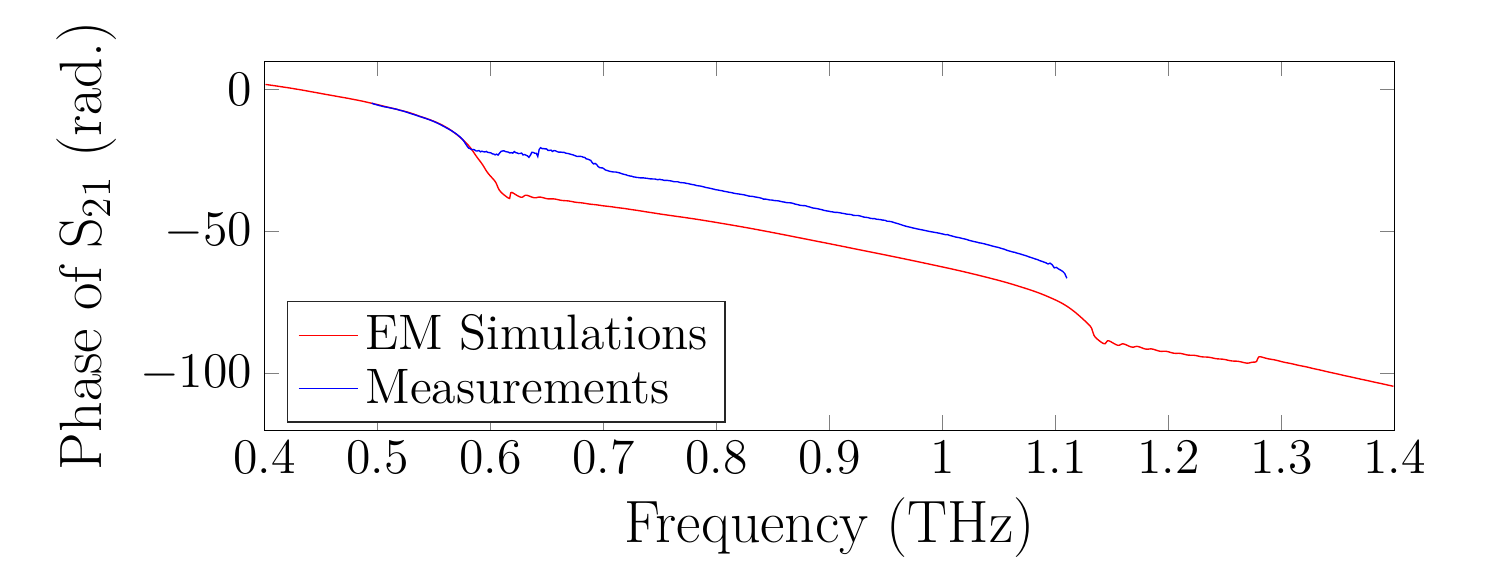}
\caption{\textbf{Five-measurement averaged S-parameters for the different liquid samples. a,b,} Magnitude of $S_{11}\text{ and }S_{22}$, respectively, having values typically bellow $\SI{xx}{dB}$. (c) Magnitude of $S_{12}\text{ and (d) }S_{21}$. Measurements within samples show high repeatability. (e) Five-sample average of phase of $S_{12}\text{ and (f) }S_{21}$, respectively.}
\label{fig:raw_sParams}
\end{figure}

In Fig.~\ref{fig:phaseVelocity_raw}a-b, single measurements of the magnitude values of $\abs{S_{12}}$ and $\abs{S_{21}}$ are plotted, giving a sense of the system's noise introduced in consecutive frequency sweeps.
The noise in both measurements is relatively low value, although it is appreciably higher for  $\abs{S_{12}}$.
The fact that $S_{22}$ and $S_{12}$ measurements are noticeable more noisier than their counterparts, $S_{11}$ and $S_{21}$, and that there is a difference in output power in the frequency extenders (Fig.~\ref{fig:DR}.b) suggests that the unequal performance of the frequency extenders yield unequal quality of measurements.
The phase velocity ($v_p=\omega/\beta$) has been plotted in Fig.~\ref{fig:phaseVelocity_raw}, which offers a frequency-adjusted value for the phase of  $\text{S}_{12}$ and  $\text{S}_{21}$. The values of phase velocity are reasonable for the refractive indexes of the materials in proximity to the CPW, and there is a consistent change of phase velocity with the IPA concentration of the sample.

\begin{figure}[h!]
\centering
\includegraphics[width=0.24\textwidth]{fig/S12_mag_allRaw.pdf}
\includegraphics[width=0.24\textwidth]{fig/S21_mag_allRaw.pdf}\\
\includegraphics[width=0.24\textwidth]{fig/phaseVelocity_raw.pdf}
\caption{\textbf{Single $S_{21}$ measurements are distinguishable in both magnitude and extracted phase velocity}. Single measurements of (a) $\abs{S_{12}}$ and (b) for each of the samples  (c) Single measurements of phase velocity for each of the samples. Both $\abs{S_{12}}$ and phase velocity values show consistent change with the sample's IPA concentration.}
\label{fig:phaseVelocity_raw}
\end{figure}



The transfer scattering matrices are related to the \mbox{S-parameters} according to \cite{Frickey1994a}:

\begin{equation*}
    [T] = \left(\begin{matrix}\frac{1}{S_{21}}&\frac{-S_{22}}{S_{21}}\\\frac{S_{11}}{S_{21}}&\frac{(S_{12}S_{21}-S_{11}S_{22})}{S_{21}}\end{matrix}\right) 
\end{equation*}



\newpage
\subsection{PDMS swelling in microfluidic channel}
The microfluidic channel, designed to be $\SI{100}{\um}$ wide, had a fabricated width of $\SI{123}{\um}$. This width wasn't affected by the sample introduced, except for pure IPA, which reduced the width to $\SI{113}{\um}$. All these dimensional changes were taken into account in our analysis.
The width of the microfluidic channel was measured with a optical microscope capable of measuring dimensions with a resolution of $\SI{1}{\um}$.
PDMS swelling has also been reported for propan-1-ol (with similar Hildebrand solubility parameter and dipolar moment as propan-2-ol) with a PDMS swelling factor of 9\%, whereas water produced no swelling \cite{Lee2003a}.
